# Supplementary material for: Automated Workflow for Absolute Binding Free Energy Calculations with Implicit Solvent and Double Decoupling
Source: arXiv:2509.21808 ancillary file (2025-09-26)
Supplement: Supplementary file 1 [file si_document.pdf]

# SI: Supporting Information for: Automated Workflow for Absolute Binding Free Energy Calculations with Implicit Solvent and Double Decoupling

Steven Ayoub<sup>\*,†,‡,||</sup> Michael Barton<sup>\*,¶,||</sup> David A. Case,<sup>§</sup> and Tyler Luchko<sup>\*,¶</sup>

<sup>†</sup>*Department of Chemistry and Biochemistry, California State University, Northridge, Northridge, CA 91330*

<sup>‡</sup>*Department of Pharmaceutical Sciences, University of California, Irvine CA 92697*

<sup>¶</sup>*Department of Physics and Astronomy, California State University, Northridge, Northridge, CA 91330*

<sup>§</sup>*Department of Chemistry and Chemical Biology, Rutgers University, Piscataway, NJ*

*|| Contributed equally to this work*

E-mail: tluchko@csun.edu

## Host Guest Systems

Figure S1 shows the cucurbit[7]uril (CB7) receptor with 14 charged guest ligands and the octa-acid (OA) receptor with 23 guest ligand host-guest systems, including the s. CB7 contains carbonyl-rich portals at the top and bottom of its cavity, which promote strong binding interactions with positively charged ammonium groups. In contrast, OA features a large, deep hydrophobic cavity of approximately 8 Å, also lined with carbonyl-rich portals, that accommodates a wide range of guest molecules.

$\alpha$ -cyclodextrin (ACD) and  $\beta$ -cyclodextrin (BCD) hosts and guest molecules are presented in Figure S2. Cyclodextrins are cyclic oligosaccharides with a hydrophobic central cavity and hydrophilic rims lined with hydroxyl groups, making them versatile hosts for a wide variety of guest molecules. ACD, with its smaller cavity, preferentially binds small linear or cyclic alcohols and amines, whereas BCD, with a larger cavity, accommodates bulkier hydrophobic guests. The figure highlights the diversity of guest molecules studied for each host, ranging from short alkyl chains to aromatic and functionalized compounds.

Figure S3 shows the water-soluble pillar[6]arene (WP6) receptor and its 13 guest molecules from the SAMPL9 dataset. WP6 is a macrocyclic molecular container composed of six phenylene units connected by methylene linkers, forming a rigid, symmetric cavity. This host exhibits high affinity for hydrophobic cationic guests, and all 13 guests studied here fall into this category<sup>1</sup>.

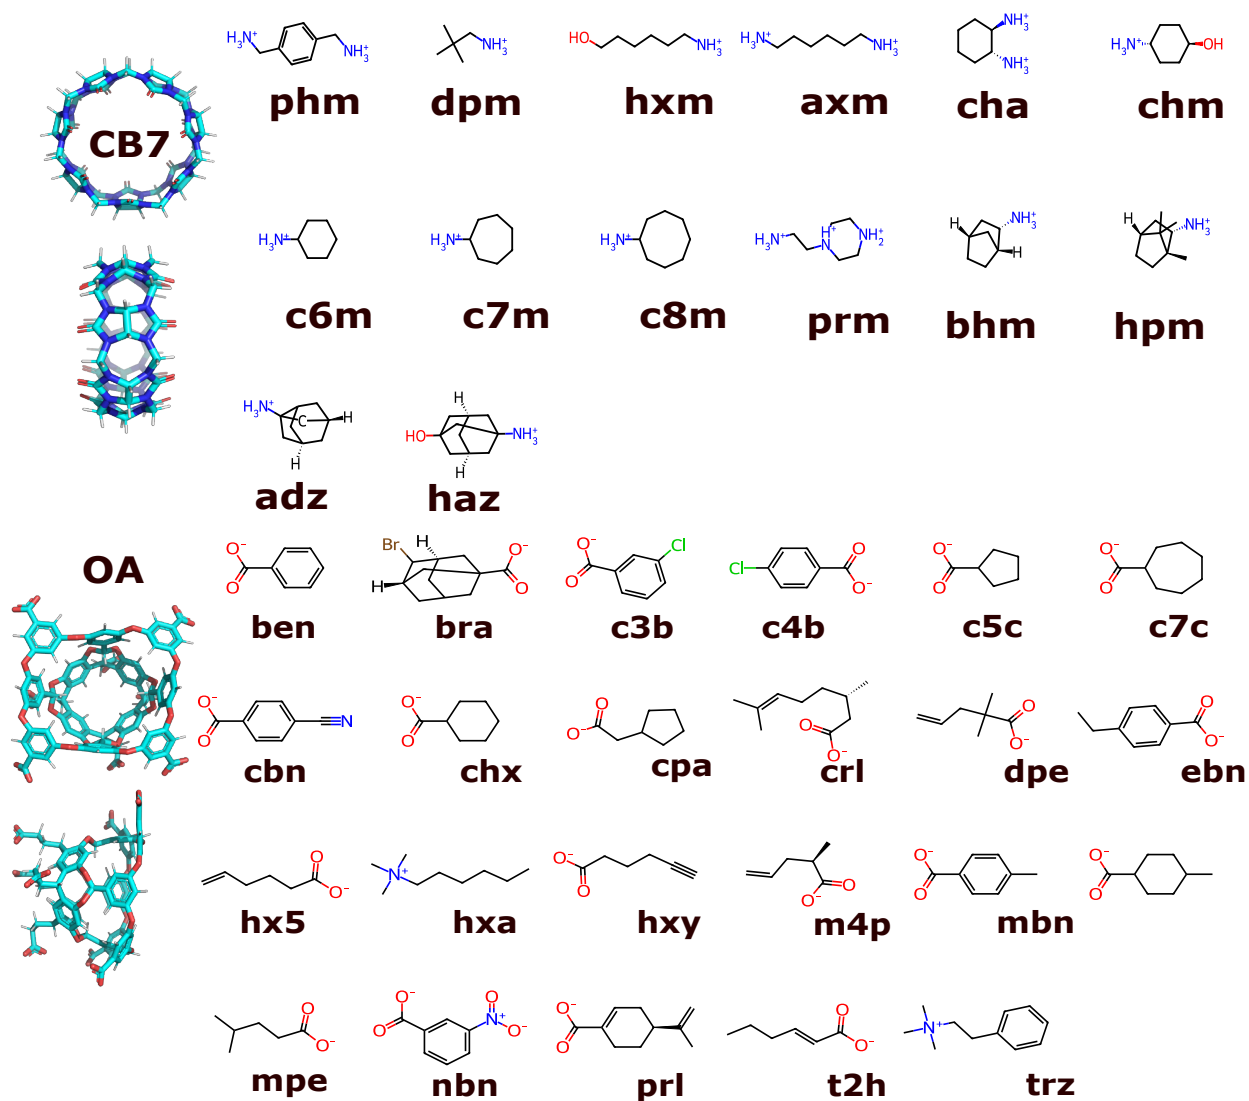

Figure S1: The dataset includes the CB7 receptor with 14 guest ligands from the SAMPL4 challenge, as well as the OA receptor with 23 guest molecules. The guest molecules are labeled using three-letter codes from Taproom<sup>2,3</sup>.

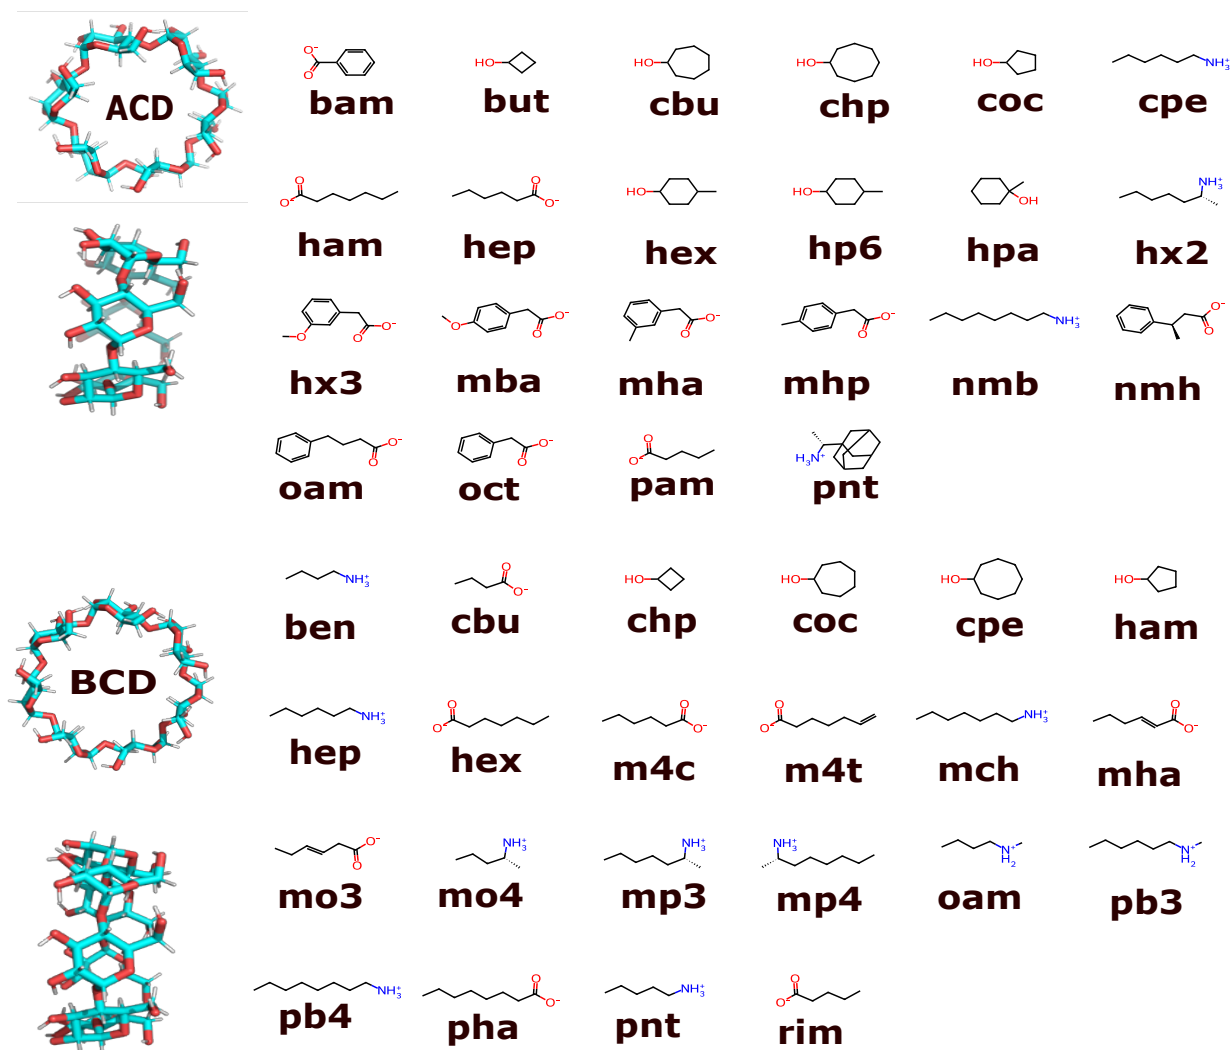

Figure S2: The dataset includes  $\alpha/\beta$ -cyclodextrins and 22 guest molecules. Each system contains 22 guest molecules labeled with three-letter codes from Taproom<sup>3</sup>, from which the structures were obtained.

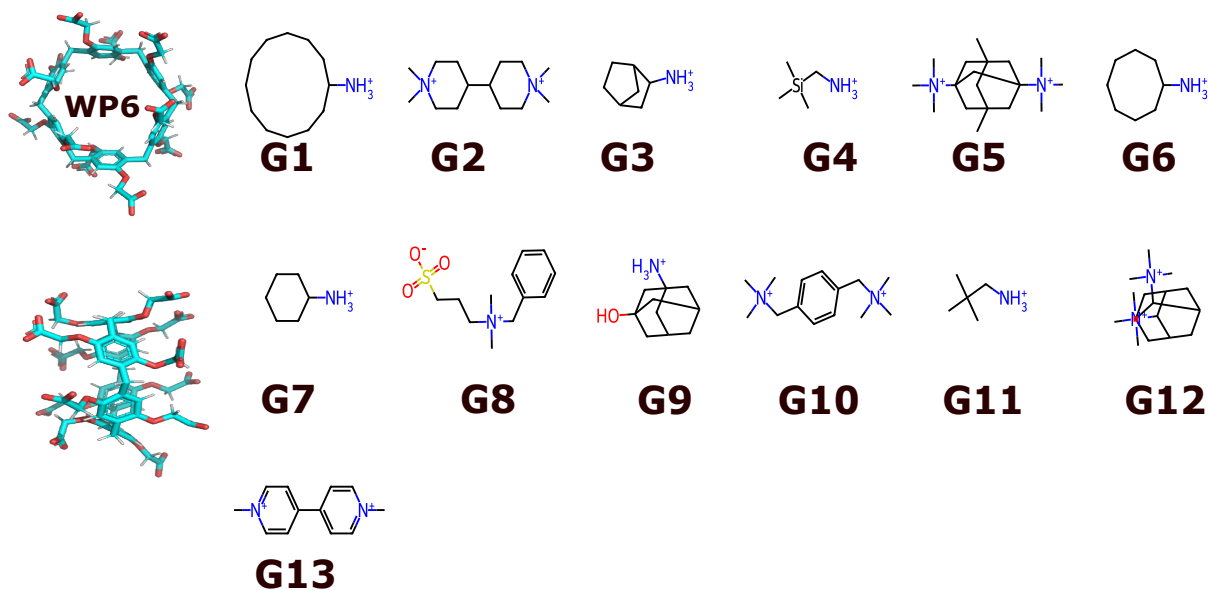

Figure S3: The dataset includes the WP6 receptor and 13 guest molecules from the SAMPL9 challenge, with structures obtained from Taproom.<sup>1,3</sup>

## Space Phase Overlap

When using perturbation approaches such as FEP or MBAR, poor phase-space overlap between neighboring states can lead to inaccurate free energy estimates. Overlap matrices provide a useful diagnostic for assessing overlap<sup>4</sup>. Each element represents the probability that a sample from state  $i$  could be observed in state  $j$ , thereby indicating the degree of configurational overlap. To obtain reliable free energy estimates, the matrix should at least be tridiagonal, with all  $(i, i + 1)$  and  $(i - 1, i)$  elements exceeding 0.03<sup>4</sup>.

The overlap matrix in Figure S4 corresponds to the complex leg of the CB7–adn system. The matrix is diagonally dominant and strongly banded, consistent with well-parameterized alchemical transitions. All nearest-neighbor elements exceed the 0.03 threshold. The lowest overlap ( $\sim 0.06$ ) occurs during the charge reintroduction step (2–3), identifying this as the most sensitive part of the cycle. In contrast, both the Lennard-Jones scaling region (0–1) and the restraint release region (7–37) maintain robust overlap values. Notably, during restraint

removal, overlaps are consistently greater than 0.2, confirming that the restraints do not create bottlenecks in sampling.

At the tail end of the restraint-release segment (19–38), we observe appreciable overlap extending beyond nearest neighbor. This suggests the  $\lambda$ -schedule in this region is likely over-resolved: adjacent states are more similar than necessary for stable reweighting. In future runs, this portion of the protocol could be thinned (e.g., removing every other  $\lambda$  in these intervals) while still maintaining the recommended nearest-neighbor overlap criterion.

| $\lambda$ | 0   | 1   | 2   | 3   | 4   | 5   | 6   | 7   | 8   | 9   | 10  | 11  | 12  | 13  | 14  | 15  | 16  | 17  | 18  | 19  | 20  | 21  | 22  | 23  | 24  | 25  | 26  | 27  | 28  | 29  | 30  | 31  | 32  | 33  | 34  | 35  | 36  | 37  | 38  |     |     |     |     |     |     |     |
|-----------|-----|-----|-----|-----|-----|-----|-----|-----|-----|-----|-----|-----|-----|-----|-----|-----|-----|-----|-----|-----|-----|-----|-----|-----|-----|-----|-----|-----|-----|-----|-----|-----|-----|-----|-----|-----|-----|-----|-----|-----|-----|-----|-----|-----|-----|-----|
| 0         | .85 | .12 | .01 | .01 | .01 |     |     |     |     |     |     |     |     |     |     |     |     |     |     |     |     |     |     |     |     |     |     |     |     |     |     |     |     |     |     |     |     |     |     |     |     |     |     |     |     |     |
| 1         | .11 | .77 | .06 | .03 | .01 | .01 |     |     |     |     |     |     |     |     |     |     |     |     |     |     |     |     |     |     |     |     |     |     |     |     |     |     |     |     |     |     |     |     |     |     |     |     |     |     |     |     |
| 2         | .01 | .07 | .31 | .29 | .18 | .07 | .05 | .02 |     |     |     |     |     |     |     |     |     |     |     |     |     |     |     |     |     |     |     |     |     |     |     |     |     |     |     |     |     |     |     |     |     |     |     |     |     |     |
| 3         | .01 | .03 | .29 | .32 | .20 | .08 | .06 | .02 |     |     |     |     |     |     |     |     |     |     |     |     |     |     |     |     |     |     |     |     |     |     |     |     |     |     |     |     |     |     |     |     |     |     |     |     |     |     |
| 4         | .01 | .02 | .17 | .20 | .27 | .19 | .11 | .03 |     |     |     |     |     |     |     |     |     |     |     |     |     |     |     |     |     |     |     |     |     |     |     |     |     |     |     |     |     |     |     |     |     |     |     |     |     |     |
| 5         |     | .01 | .08 | .09 | .23 | .37 | .18 | .03 |     |     |     |     |     |     |     |     |     |     |     |     |     |     |     |     |     |     |     |     |     |     |     |     |     |     |     |     |     |     |     |     |     |     |     |     |     |     |
| 6         |     | .01 | .05 | .06 | .11 | .16 | .35 | .21 | .05 |     |     |     |     |     |     |     |     |     |     |     |     |     |     |     |     |     |     |     |     |     |     |     |     |     |     |     |     |     |     |     |     |     |     |     |     |     |
| 7         |     |     | .02 | .02 | .03 | .03 | .22 | .38 | .25 | .04 | .01 |     |     |     |     |     |     |     |     |     |     |     |     |     |     |     |     |     |     |     |     |     |     |     |     |     |     |     |     |     |     |     |     |     |     |     |
| 8         |     |     |     |     | .05 | .24 | .42 | .20 | .07 | .01 |     |     |     |     |     |     |     |     |     |     |     |     |     |     |     |     |     |     |     |     |     |     |     |     |     |     |     |     |     |     |     |     |     |     |     |     |
| 9         |     |     |     |     |     | .06 | .27 | .33 | .27 | .06 | .01 |     |     |     |     |     |     |     |     |     |     |     |     |     |     |     |     |     |     |     |     |     |     |     |     |     |     |     |     |     |     |     |     |     |     |     |
| 10        |     |     |     |     |     | .01 | .07 | .21 | .40 | .22 | .09 | .01 |     |     |     |     |     |     |     |     |     |     |     |     |     |     |     |     |     |     |     |     |     |     |     |     |     |     |     |     |     |     |     |     |     |     |
| 11        |     |     |     |     |     |     | .01 | .05 | .25 | .31 | .28 | .08 |     |     |     |     |     |     |     |     |     |     |     |     |     |     |     |     |     |     |     |     |     |     |     |     |     |     |     |     |     |     |     |     |     |     |
| 12        |     |     |     |     |     |     |     | .01 | .07 | .20 | .41 | .28 | .03 |     |     |     |     |     |     |     |     |     |     |     |     |     |     |     |     |     |     |     |     |     |     |     |     |     |     |     |     |     |     |     |     |     |
| 13        |     |     |     |     |     |     |     |     | .01 | .07 | .30 | .46 | .16 | .01 |     |     |     |     |     |     |     |     |     |     |     |     |     |     |     |     |     |     |     |     |     |     |     |     |     |     |     |     |     |     |     |     |
| 14        |     |     |     |     |     |     |     |     |     | .03 | .16 | .60 | .19 | .01 |     |     |     |     |     |     |     |     |     |     |     |     |     |     |     |     |     |     |     |     |     |     |     |     |     |     |     |     |     |     |     |     |
| 15        |     |     |     |     |     |     |     |     |     |     | .01 | .20 | .55 | .22 | .02 |     |     |     |     |     |     |     |     |     |     |     |     |     |     |     |     |     |     |     |     |     |     |     |     |     |     |     |     |     |     |     |
| 16        |     |     |     |     |     |     |     |     |     |     |     | .01 | .22 | .49 | .23 | .04 |     |     |     |     |     |     |     |     |     |     |     |     |     |     |     |     |     |     |     |     |     |     |     |     |     |     |     |     |     |     |
| 17        |     |     |     |     |     |     |     |     |     |     |     |     | .02 | .23 | .42 | .25 | .06 | .01 |     |     |     |     |     |     |     |     |     |     |     |     |     |     |     |     |     |     |     |     |     |     |     |     |     |     |     |     |
| 18        |     |     |     |     |     |     |     |     |     |     |     |     |     | .04 | .23 | .40 | .23 | .07 | .02 | .01 |     |     |     |     |     |     |     |     |     |     |     |     |     |     |     |     |     |     |     |     |     |     |     |     |     |     |
| 19        |     |     |     |     |     |     |     |     |     |     |     |     |     |     | .06 | .25 | .32 | .21 | .10 | .04 | .01 |     |     |     |     |     |     |     |     |     |     |     |     |     |     |     |     |     |     |     |     |     |     |     |     |     |
| 20        |     |     |     |     |     |     |     |     |     |     |     |     |     |     |     | .01 | .09 | .22 | .26 | .20 | .12 | .06 | .03 | .01 |     |     |     |     |     |     |     |     |     |     |     |     |     |     |     |     |     |     |     |     |     |     |
| 21        |     |     |     |     |     |     |     |     |     |     |     |     |     |     |     |     | .02 | .10 | .19 | .22 | .19 | .13 | .07 | .03 | .01 | .01 | .01 |     |     |     |     |     |     |     |     |     |     |     |     |     |     |     |     |     |     |     |
| 22        |     |     |     |     |     |     |     |     |     |     |     |     |     |     |     |     |     | .01 | .04 | .11 | .18 | .20 | .18 | .12 | .07 | .03 | .03 | .02 | .01 | .01 |     |     |     |     |     |     |     |     |     |     |     |     |     |     |     |     |
| 23        |     |     |     |     |     |     |     |     |     |     |     |     |     |     |     |     |     |     | .01 | .05 | .12 | .17 | .19 | .15 | .10 | .06 | .05 | .03 | .02 | .01 | .01 | .01 | .01 |     |     |     |     |     |     |     |     |     |     |     |     |     |
| 24        |     |     |     |     |     |     |     |     |     |     |     |     |     |     |     |     |     |     |     | .03 | .07 | .13 | .17 | .15 | .12 | .08 | .07 | .05 | .04 | .02 | .02 | .01 | .01 | .01 | .01 | .01 |     |     |     |     |     |     |     |     |     |     |
| 25        |     |     |     |     |     |     |     |     |     |     |     |     |     |     |     |     |     |     |     |     | .01 | .04 | .09 | .13 | .14 | .12 | .09 | .09 | .07 | .06 | .04 | .03 | .02 | .02 | .02 | .02 | .01 | .01 | .01 | .01 |     |     |     |     |     |     |
| 26        |     |     |     |     |     |     |     |     |     |     |     |     |     |     |     |     |     |     |     |     |     | .01 | .02 | .05 | .09 | .11 | .11 | .09 | .10 | .08 | .08 | .05 | .05 | .03 | .03 | .03 | .03 | .02 | .02 | .02 | .01 |     |     |     |     |     |
| 27        |     |     |     |     |     |     |     |     |     |     |     |     |     |     |     |     |     |     |     |     |     |     | .01 | .03 | .06 | .08 | .09 | .08 | .10 | .09 | .09 | .07 | .07 | .04 | .04 | .04 | .04 | .03 | .03 | .02 | .02 |     |     |     |     |     |
| 28        |     |     |     |     |     |     |     |     |     |     |     |     |     |     |     |     |     |     |     |     |     |     |     | .01 | .02 | .04 | .05 | .06 | .06 | .09 | .09 | .10 | .08 | .08 | .06 | .06 | .05 | .04 | .04 | .04 | .03 |     |     |     |     |     |
| 29        |     |     |     |     |     |     |     |     |     |     |     |     |     |     |     |     |     |     |     |     |     |     |     |     | .01 | .02 | .04 | .05 | .05 | .08 | .08 | .10 | .08 | .09 | .07 | .07 | .07 | .06 | .05 | .05 | .04 |     |     |     |     |     |
| 30        |     |     |     |     |     |     |     |     |     |     |     |     |     |     |     |     |     |     |     |     |     |     |     |     |     | .01 | .02 | .02 | .03 | .04 | .06 | .07 | .09 | .08 | .10 | .07 | .08 | .08 | .07 | .06 | .06 | .05 |     |     |     |     |
| 31        |     |     |     |     |     |     |     |     |     |     |     |     |     |     |     |     |     |     |     |     |     |     |     |     |     |     | .01 | .02 | .02 | .03 | .05 | .06 | .09 | .08 | .10 | .08 | .09 | .09 | .08 | .07 | .07 | .06 |     |     |     |     |
| 32        |     |     |     |     |     |     |     |     |     |     |     |     |     |     |     |     |     |     |     |     |     |     |     |     |     |     |     | .01 | .01 | .02 | .02 | .04 | .06 | .08 | .08 | .10 | .08 | .09 | .09 | .08 | .08 | .08 | .08 |     |     |     |
| 33        |     |     |     |     |     |     |     |     |     |     |     |     |     |     |     |     |     |     |     |     |     |     |     |     |     |     |     |     | .01 | .01 | .01 | .02 | .04 | .05 | .07 | .07 | .09 | .08 | .09 | .10 | .09 | .09 | .09 |     |     |     |
| 34        |     |     |     |     |     |     |     |     |     |     |     |     |     |     |     |     |     |     |     |     |     |     |     |     |     |     |     |     |     | .01 | .01 | .02 | .03 | .04 | .06 | .06 | .09 | .07 | .09 | .10 | .09 | .10 | .12 |     |     |     |
| 35        |     |     |     |     |     |     |     |     |     |     |     |     |     |     |     |     |     |     |     |     |     |     |     |     |     |     |     |     |     |     | .01 | .01 | .01 | .03 | .04 | .06 | .06 | .08 | .07 | .09 | .10 | .10 | .10 | .14 |     |     |
| 36        |     |     |     |     |     |     |     |     |     |     |     |     |     |     |     |     |     |     |     |     |     |     |     |     |     |     |     |     |     |     |     | .01 | .01 | .02 | .03 | .05 | .05 | .07 | .07 | .09 | .10 | .10 | .11 | .12 | .16 |     |
| 37        |     |     |     |     |     |     |     |     |     |     |     |     |     |     |     |     |     |     |     |     |     |     |     |     |     |     |     |     |     |     |     |     | .01 | .01 | .02 | .03 | .04 | .05 | .07 | .06 | .09 | .10 | .11 | .11 | .12 | .18 |
| 38        |     |     |     |     |     |     |     |     |     |     |     |     |     |     |     |     |     |     |     |     |     |     |     |     |     |     |     |     |     |     |     |     |     | .01 | .01 | .02 | .03 | .03 | .05 | .05 | .08 | .10 | .11 | .12 | .14 | .24 |

Figure S4: Overlap matrix for the CB7–adn complex using the OBC model. State indices (x- and y-axis) correspond to the full complex leg of the alchemical cycle, ranging from state 0 (no host–guest interactions, restraints active) to state 38 (fully interacting host and guest, restraints removed). In states 1–2, Lennard-Jones interactions are turned on. States 3–4 scale the ligand electrostatics from 50% to full charges. Lambda states 5–6 scale the generalized Born (GB) dielectric constant from 10% to 100%. Finally, lambda states 7–37 progressively remove both conformational and orientational restraints.

## References

- (1) Amezcua, M.; Setiadi, J.; Mobley, D. L. The SAMPL9 host-guest blind challenge: an overview of binding free energy predictive accuracy. *Phys. Chem. Chem. Phys.* **2024**, *26*, 9207–9225.
- (2) Muddana, H. S.; Fenley, A. T.; Mobley, D. L.; Gilson, M. K. The SAMPL4 host-guest blind prediction challenge: an overview. *Journal of Computer-Aided Molecular Design* **2014**, *28*, 305–317.
- (3) Slochower, D. Taproom. 2022.
- (4) Klimovich, P. V.; Shirts, M. R.; Mobley, D. L. Guidelines for the analysis of free energy calculations. *Journal of Computer-Aided Molecular Design* **2015**, *29*, 397–411.
